# Supplementary material for: SAG-ViT: A Scale-Aware, High-Fidelity Patching Approach with Graph Attention for Vision Transformers
Source: arXiv:2411.09420 source file (2025-01-08)
Supplement: Supplementary file 1 [file X_suppl.tex]

\clearpage
\setcounter{page}{1}
\maketitlesupplementary

\subsection{Ablation Study}

To rigorously evaluate the contributions of each component in our proposed architecture, we conducted a comprehensive ablation study. This analysis aims to discern the individual impact of the EfficientNet backbone, the Graph Attention Network (GAT), and the Transformer encoder on the model's overall performance. By systematically removing or altering components, we can quantify their significance and validate the theoretical underpinnings of our design choices.

\subsubsection{Experimental Setup}

We designed three ablation experiments on the CIFAR-10 dataset to isolate the effects of each component:

\begin{enumerate}
    \item \textbf{Backbone + GAT (No Transformer):} In this configuration, we exclude the Transformer encoder, allowing us to assess the role of the Transformer in capturing global dependencies. The model processes the feature embeddings extracted by the EfficientNet backbone through the GAT, generating class predictions directly from the aggregated node representations.

    \item \textbf{Backbone + Transformer (No GAT):} Here, we omit the GAT to evaluate its contribution in modeling local dependencies and refining node features. The feature embeddings from the backbone are fed into the Transformer encoder, which attempts to learn both local and global relationships without the explicit attention mechanism provided by the GAT.

    \item \textbf{GAT + Transformer (No Backbone):} In this scenario, we remove the EfficientNet backbone to determine its impact on feature representation. Randomly initialized embeddings are used as input to the GAT and Transformer, highlighting the importance of high-quality feature extraction.
\end{enumerate}

\subsection{Results and Discussion}

\begin{table*}[h]
    \centering
    \caption{Ablation Study Results on Benchmark Datasets}
    \label{tab:ablation_study}
    \input{sec/table3} 
\end{table*}

When the model includes the EfficientNet backbone with the GAT but without the Transformer encoder, the F1 score drops to 0.7785. This significant decrease underscores the crucial role of the Transformer encoder in capturing global dependencies and enhancing classification accuracy. The self-attention mechanism in the Transformer allows the model to weigh the importance of all patches relative to each other, facilitating a holistic understanding of the image.

Conversely, using the EfficientNet backbone with the Transformer encoder but without the GAT results in an F1 score of 0.7593. This emphasizes the importance of the GAT in refining local feature representations before global processing. The GAT enhances node features by aggregating information from immediate neighbors, effectively capturing local structural information essential for accurate classification.

When the model comprises the GAT and Transformer encoder without the EfficientNet backbone, the F1 score drops drastically to 0.5032. This significant decline highlights the importance of the EfficientNet backbone in providing rich and discriminative feature embeddings necessary for effective graph construction and subsequent processing. The results are summarized in Table~\ref{tab:ablation_study}. The RAM and GPU VRAM usage of various models are illustrated in Figure~\ref{fig:ablationFig}.

\begin{figure}[t]
  \centering
   \includegraphics[width=1\linewidth]{sec/ablation_top_right_legend.png}

   \caption{Ablation study of model configurations, showing F1 Score, RAM, and GPU VRAM usage (GB) for different combinations of backbone, GAT, and Transformer components.}
   \label{fig:ablationFig}
\end{figure}

These observations confirm that each component of our proposed architecture is essential and contributes uniquely to the model's overall performance. The EfficientNet backbone generates high-quality feature embeddings; the GAT captures local dependencies through attention mechanisms; and the Transformer encoder models global relationships, enabling the model to understand complex patterns that span different regions of the image.
